# Supplementary material for: Semi-Truths: A Large-Scale Dataset of AI-Augmented Images for Evaluating Robustness of AI-Generated Image detectors
Source: arXiv:2411.07472 source file (2024-11-12)
Supplement: Supplementary file 1 [file appendix_crop_algo.tex]

\begin{algorithm}
\caption{An algorithm with caption}\label{alg:cap}
\begin{algorithmic}[1]
\Require $n \geq 0$
\Ensure $y = x^n$
\State $y \gets 1$
\State $X \gets x$
\State $N \gets n$
\While{$N \neq 0$}
\If{$N$ is even}
    \State $X \gets X \times X$
    \State $N \gets \frac{N}{2}$  \Comment{This is a comment}
\ElsIf{$N$ is odd}
    \State $y \gets y \times X$
    \State $N \gets N - 1$
\EndIf
\EndWhile
\end{algorithmic}
\end{algorithm}
